# Supplementary material for: Delta Denoising Score
Source: arXiv:2304.07090 source file (2023-04-14)
Supplement: Supplementary file 1 [file tex_supp_net_result_figures.tex]

\begin{figure*}
\centering
    \includegraphics[width=\textwidth]{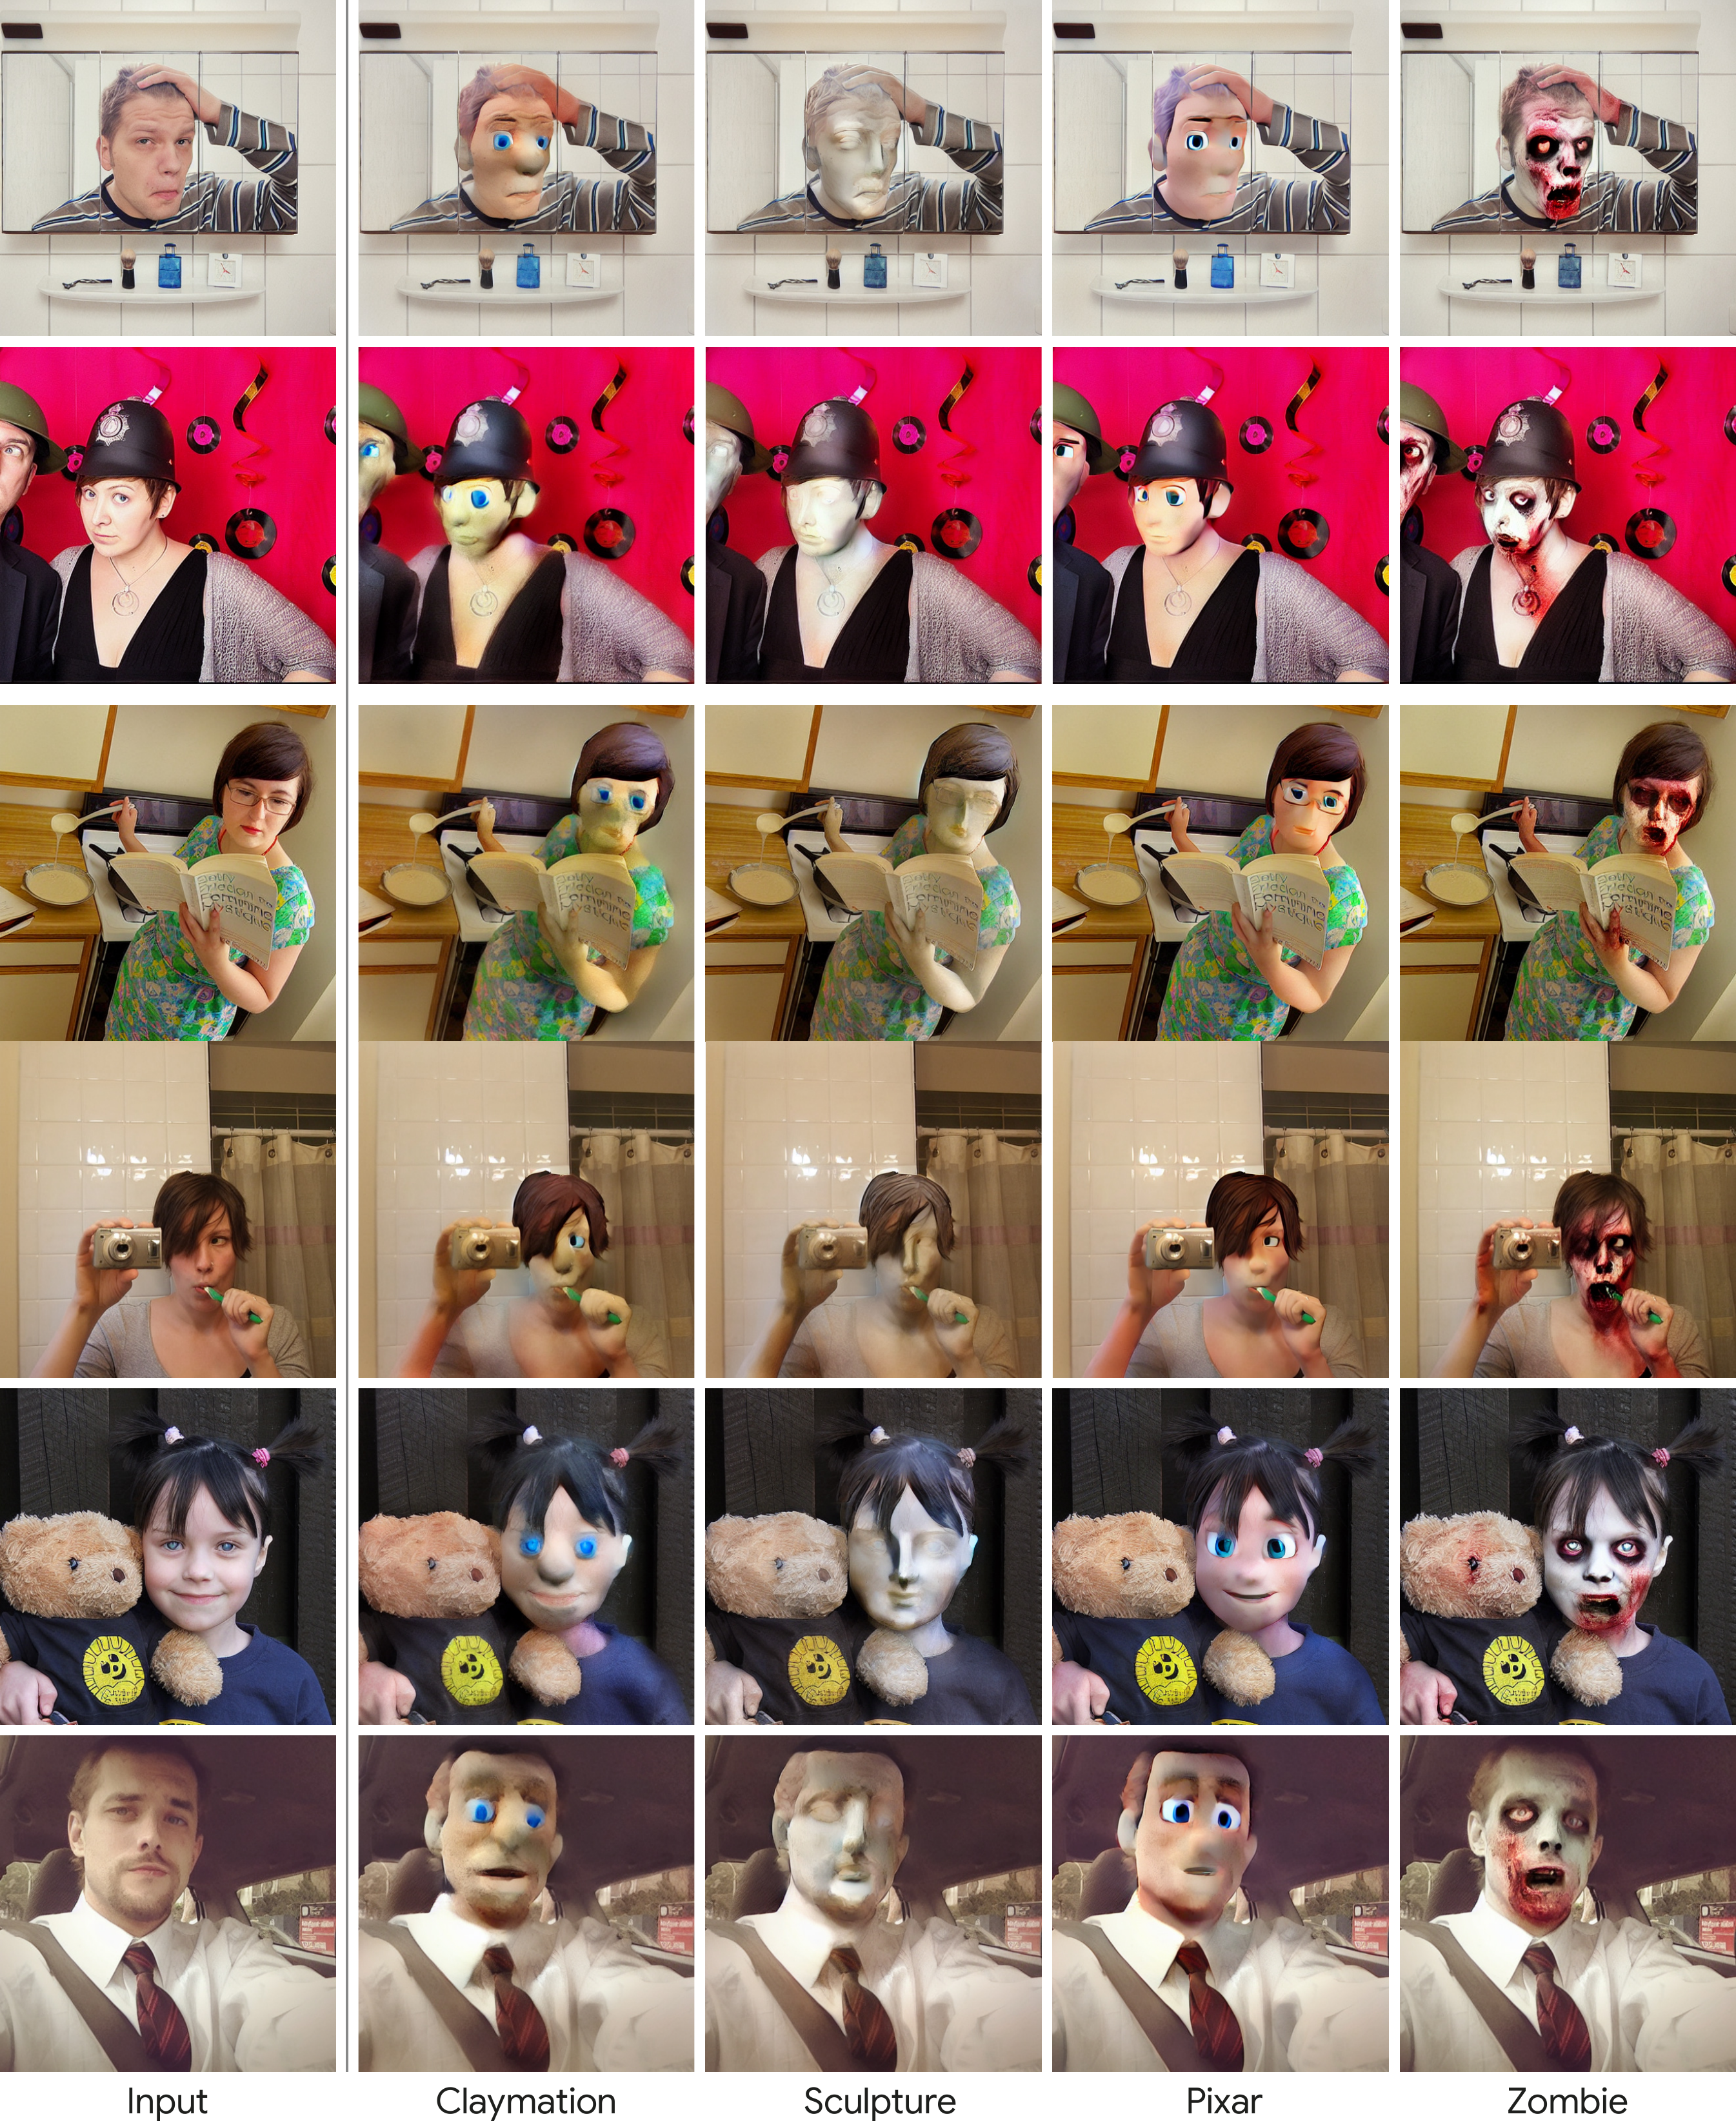}
    \caption{\bf{Unsupervised image-to-image translation-- characters.} {\it Different networks were trained to change the person in the image to various characters.
    The networks were trained on FFHQ in-the-wild dataset (unaligned) \cite{karras2019style} and tested on images from COCO dataset \cite{caesar2018coco}.}}
    \label{fig:supp_characters1}
\end{figure*}
